# Supplementary material for: SPARTA: Evaluating Reasoning Segmentation Robustness through Black-Box Adversarial Paraphrasing in Text Autoencoder Latent Space
Source: arXiv:2510.24446 source file (2025-10-28)
Supplement: Supplementary file 1 [file sp-simple.tex]

\begin{figure}[t!]
  \centering
  \includegraphics[width=0.5\linewidth]{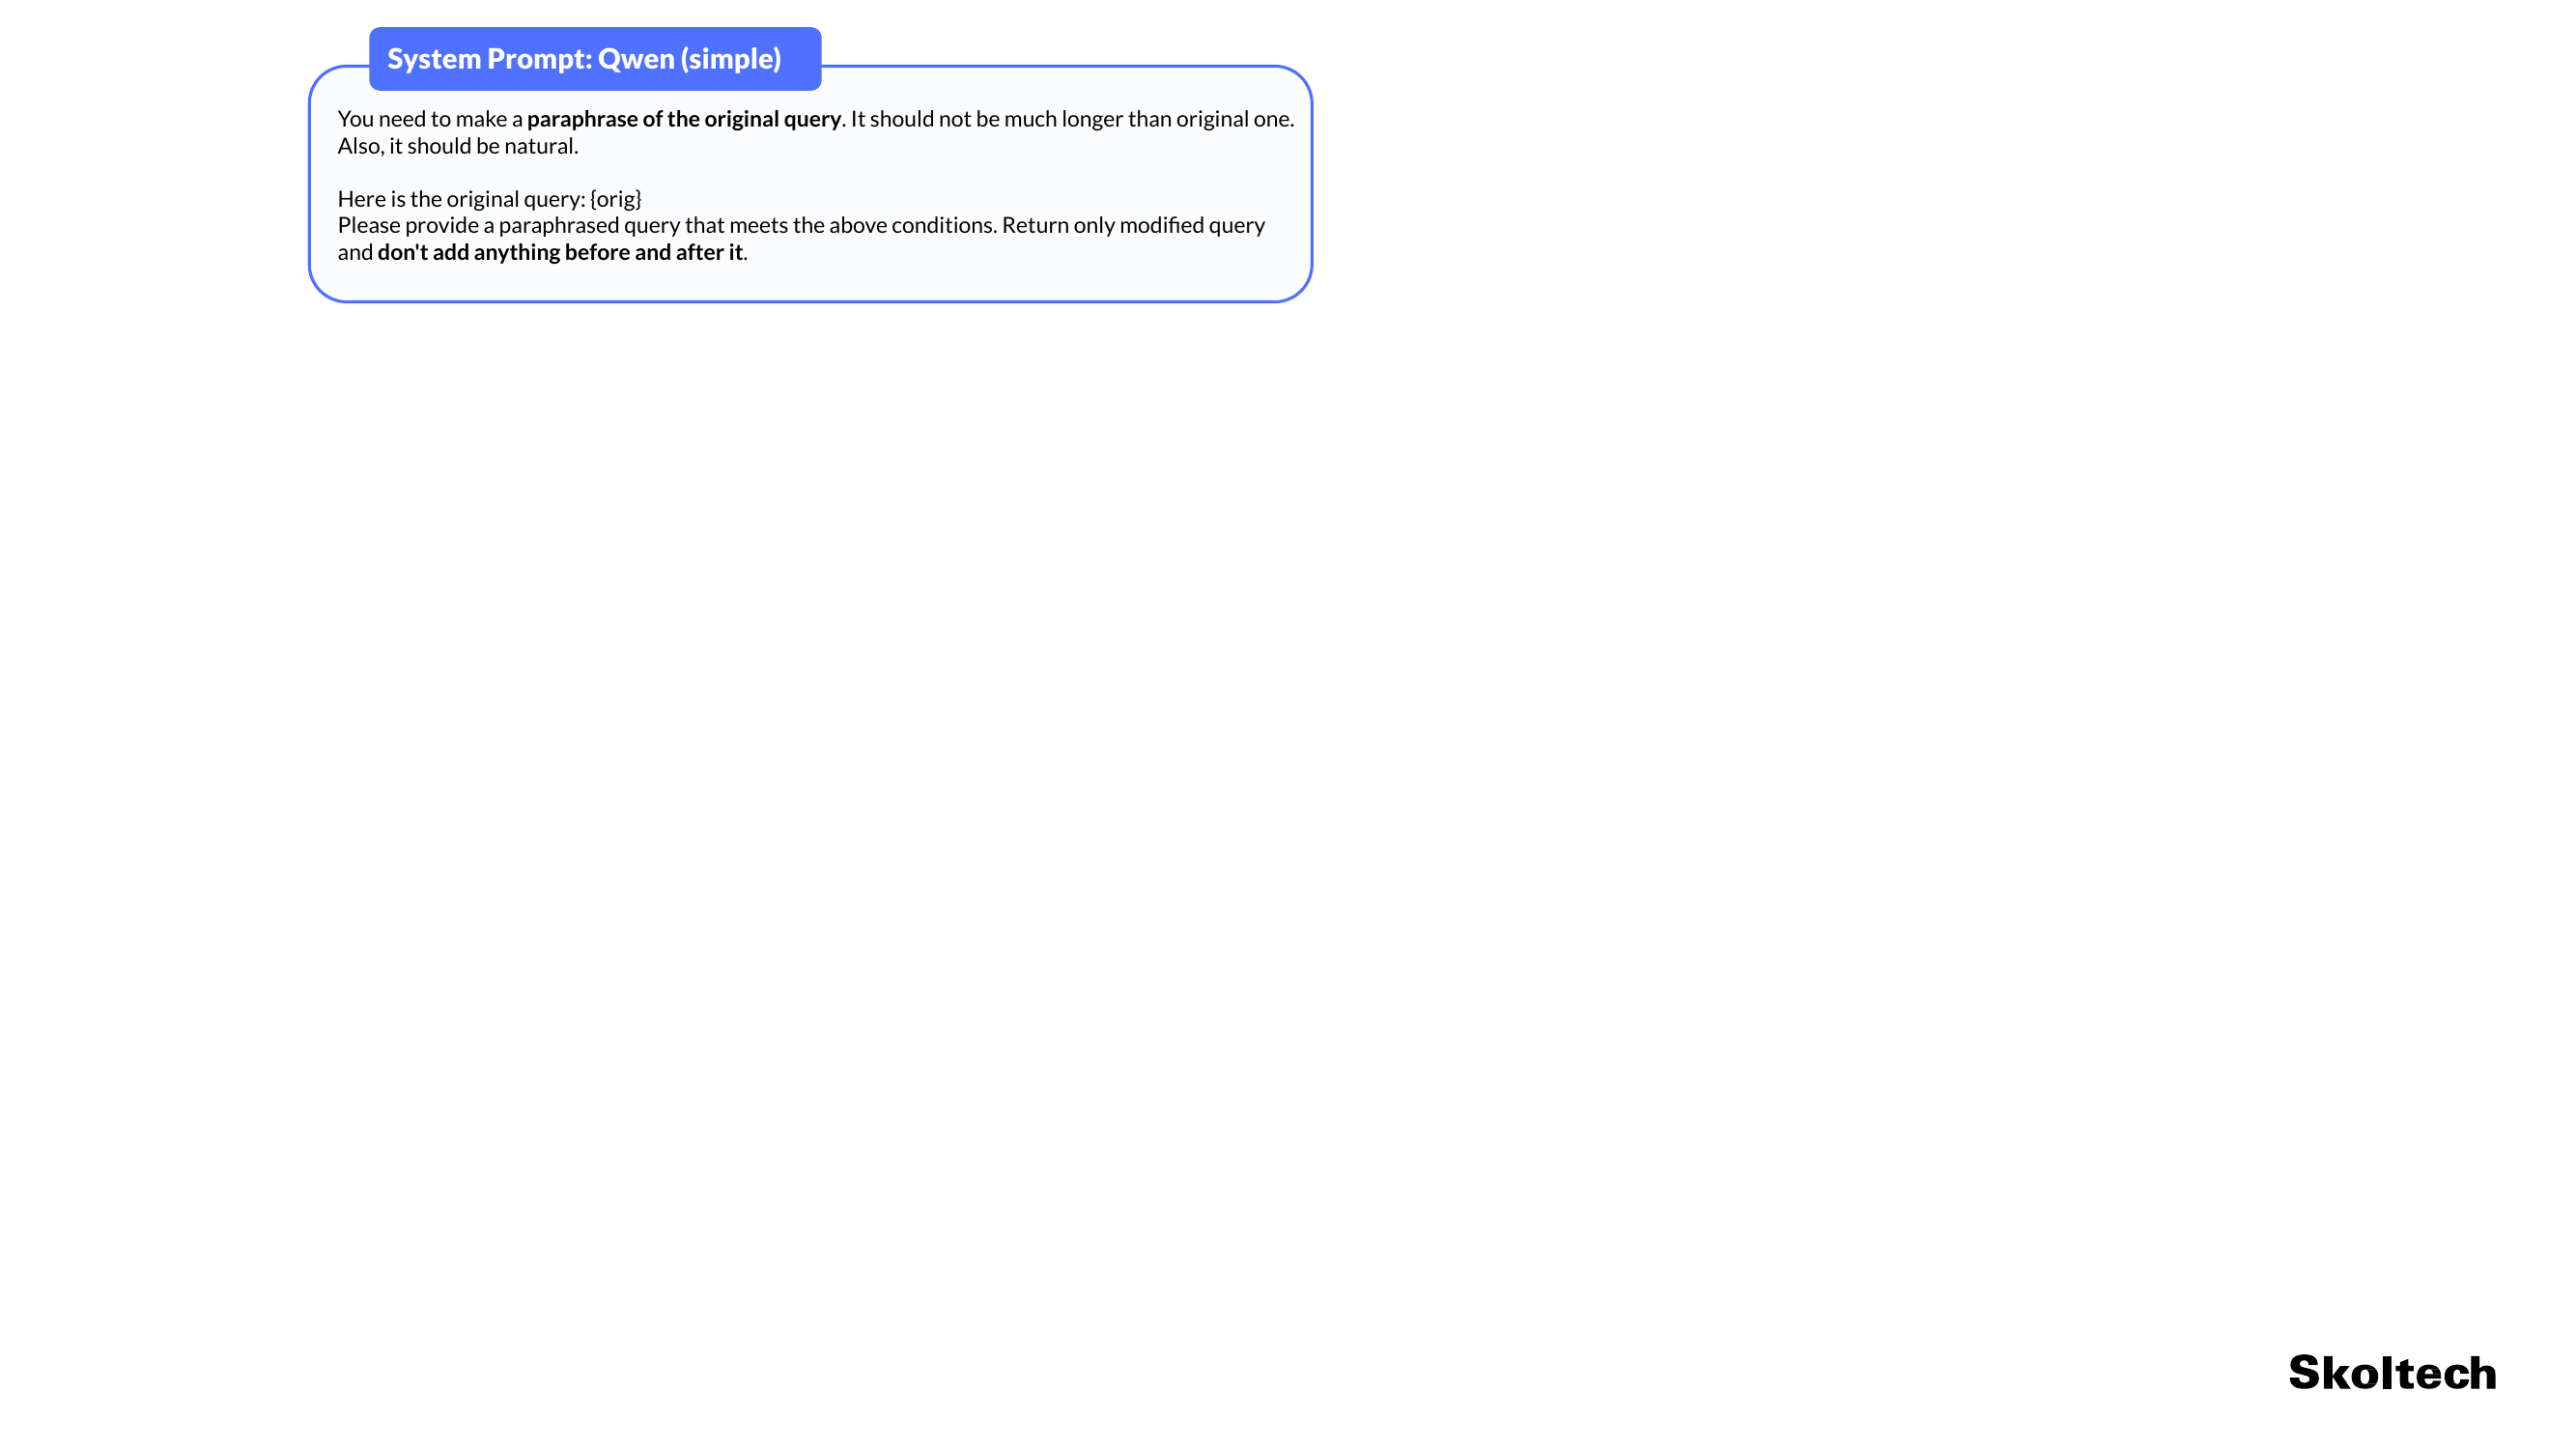}
    \captionsetup{type=figure}
  \caption{\textbf{System Prompt} employed in Qwen3-32B \textit{simple} prompt attack.}
\label{table:prompt_simple}
\end{figure}
