# Supplementary material for: SPARTA: Evaluating Reasoning Segmentation Robustness through Black-Box Adversarial Paraphrasing in Text Autoencoder Latent Space
Source: arXiv:2510.24446 source file (2025-10-28)
Supplement: Supplementary file 3 [file llm_scoring.tex]

\section{LLM-scoring}

\subsection{Prompt}

\input{supplement/tables/system_prompt}

For nvidia/Llama-3.1-Nemotron-70B-Instruct-HF~\cite{wang2024helpsteer2preferencecomplementingratingspreferences} we used the system prompt in Table \ref{table:system_prompt}.



\subsection{Human Assessment}
\label{app:hs}

One approach to score paraphrases is a binary human assessment, where experts confirm whether a paraphrase is valid.
However, this is costly to scale.
Thus, we rely on an LLM-based assessment to approximate human judgment, in line with findings from~\cite{fu-etal-2024-gptscore, wang-etal-2023-chatgpt, chiang-lee-2023-large, chan2023chateval}.

\input{supplement/tables/instruction}

To validate LLM-based scoring for our specific task, we first evaluated its alignment with human annotations.
We curated a balanced dataset of 200 adversarial paraphrases, comprising 100 pairs from GBDA and 100 from RText to mitigate attack-specific bias.
Within each subset, 50 pairs had received a perfect LLM-score (5/5) and 50 had received a lower score, reflecting our observation that LLMs frequently assign perfect scores to many high-quality paraphrases.
This 50/50 split was applied independently to the GBDA and RText portions, yielding a dataset that is balanced not only across attack types but also across LLM-score bands.
Authors of the paper fluent in English assessed these paraphrases for grammatical and syntactical correctness, as well as semantic equivalence, according to the instructions provided in Table~\ref{table:instruction}.
For prompt selection, we binarized the LLM outputs: perfect scores were mapped to 1 (indicating a valid paraphrase) and all other scores to 0.
Framing this as a binary classification task, we calculated the F1-score as a compromise metric between precision and recall.
The resulting metric \text{F1-score} = 0.87 affirm a strong alignment between LLM and expert assessments.
