# Supplementary material for: SPARTA: Evaluating Reasoning Segmentation Robustness through Black-Box Adversarial Paraphrasing in Text Autoencoder Latent Space
Source: arXiv:2510.24446 source file (2025-10-28)
Supplement: Supplementary file 4 [file instruction.tex]

\begin{table}[t!]  
\centering
\captionsetup{type=table} % Force caption type
\begin{lstlisting}[language=,escapeinside={(*}{*)}]
You'll receive two sentences: the Original and its Paraphrase.
Return a single digit:

1 - Paraphrase is both grammatically and syntactically correct 
AND means exactly the same as the Original.
0 - Otherwise (any grammatical, syntactical error or meaning
change/addition/omission).

Example 1
Original: "What object would people sit on when eating 
together at a dining table?"
Paraphrase: "On what object would people sit when eating 
together at a dining table?"
Return: 1

Example 2
Original: "What object would people sit on when eating 
together at a dining table?"
Paraphrase: "On what object would people (*\textbf{stand}*) when eating 
together at a dining table?"
Return: 0

Example 3
Original: "What object would people sit on when eating 
together at a dining table?"
Paraphrase: "What object would people sit on when (*\textbf{aating}*) 
together at a dining table?"
Return: 0
\end{lstlisting}
\caption{Instruction for annotators.}
\label{table:instruction}
\end{table}
