# Supplementary material for: SPARTA: Evaluating Reasoning Segmentation Robustness through Black-Box Adversarial Paraphrasing in Text Autoencoder Latent Space
Source: arXiv:2510.24446 source file (2025-10-28)
Supplement: Supplementary file 6 [file system_prompt_adv.tex]

\begin{table}[t!]  
\centering
\captionsetup{type=table} % Force caption type
\tiny 

\begin{lstlisting}[language=,numbers=none,breaklines=true,breakatwhitespace=true,breakindent=0pt,postbreak=\mbox{}]
You are tasked with subtly altering a query for a reasoning segmentation system. The system is designed to output a segmentation mask based on the query text and an image. Your goal is to slightly modify the query so that:
1. The text remains grammatically correct and plausible.
2. The modified query refers to the same general concept or object but introduces subtle ambiguities or misleading details that can cause the system to generate an incorrect segmentation mask.
3. The meaning is implicit and still related to the original context but exploits the reasoning weakness of the system.
Here is the original query:
{orig}
Please provide a subtly modified query that meets the above conditions.
Return only modified query and don't add anything before and after it.
\end{lstlisting}
\caption{\textbf{System Prompt} employed in Qwen3 simple prompt attack.}
\label{table:prompt_adv}

\end{table}
