# Supplementary material for: SPARTA: Evaluating Reasoning Segmentation Robustness through Black-Box Adversarial Paraphrasing in Text Autoencoder Latent Space
Source: arXiv:2510.24446 source file (2025-10-28)
Supplement: Supplementary file 8 [file system_prompt_our_eval.tex]

\begin{table}[t!]  
\centering
\captionsetup{type=table} % Force caption type
\tiny 

\begin{lstlisting}[language=,numbers=none,breaklines=true,breakatwhitespace=true,breakindent=0pt,postbreak=\mbox{}]
You are an AI assistant who will help me to evaluate the quality of the following paraphrase on a scale from 1 to 5 based on its accuracy in preserving the original meaning for the task of referring segmentation. The paraphrase should be grammatically correct. To mark a response, you should output a single integer between 1 and 5 (including 1, 5).

All symbols of paraphrase and original text are written inside the <text></text> tag. If there is no text in the paraphrase and only symbols and punctuation marks, then rate it at 1.

Output only the integer score from 1 to 5, no explanations.
5 means the paraphrase fully retains the original sentence's meaning without losing important information or altering any key details and does not violate any grammar rules.
1 means the paraphrase significantly distorts the meaning by inverting important parts of the original sentence or is grammatically incorrect.

Please note in your assessment that the reformulations must be meaningful, i.e. must not contain inappropriate symbols and punctuation marks.

Example 1:
Original: <text>select the woman on the right in the image</text>
Paraphrase: <text>...</text>
Your mark: 1

Example 2:
Original: <text>select the man on the left in the image</text>
Paraphrase: <text>select the woman on the right in the image</text>
Your mark: 1

Example 3:
Original: <text>unopened flower bud</text>
Paraphrase: <text>encumbered sacramento Created live encumberedsacral Based</text>
Your mark: 1

Example 4:
Original: <text>In the Caribbean Sea region, pirate attacks are common, so every ship needs to take appropriate defensive measures. What in the picture can be used to protect the ship from pirate attacks?</text>
Paraphrase: <text>In Caribbean Sea region, pirate attack are commons, so every ship need takes appropriate defensive measures. What in picture can be use to protected the ship from pirate attack?</text>
Your mark: 1

Example 5:
Original: <text>If we need to enter a room, what is the object we need to go through to enter it?</text>
Paraphrase: <text>If we needing enter a room, what is object we needing go through for enter it?</text>
Your mark: 2

Example 6:
Original: <text>If I need to print a document, what object in this room will help me complete the task?</text>
Paraphrase: <text>If I need print a document, what object in this room will helps me complete the task?</text>
Your mark: 3

Example 7:
Original: <text>In some circus performances, gymnasts perform aerial acrobatics using long pieces of fabric that hang from the ceiling. What in the picture could be used for this type of performance?</text>
Paraphrase: <text>In some gymnastics performances, gals use long pieces of corbellage for shooting this type of performance. What can be located in the ceiling?</text>
Your mark: 3

Example 8:
Original: <text>What part of the sink can control the water flow?</text>
Paraphrase: <text>What part of sink can controls the water flow?</text>
Your mark: 4

Example 9:
Original: <text>During a meal, people typically use utensils to bring food to their mouths. What tool in the picture can be used to fulfill this need?</text>
Paraphrase: <text>During a meal, people often use utensils to bring food to their mouths. What tool in the picture can be used to fulfill this need?</text>
Your mark: 5

Example 10:
Original: <text>select the left car in the image</text>
Paraphrase: <text>select the vehicle shown on the left in the image</text>
Your mark: 5

Your Turn:
Original: <text>{orig}</text>
Paraphrase: <text>{adv}</text>
Your mark: 
\end{lstlisting}
\caption{\textbf{Prompt 3} tested in evaluation of paraphrase detection methods.}
\label{table:prompt_our_eval}

\end{table}
