# Supplementary material for: SPARTA: Evaluating Reasoning Segmentation Robustness through Black-Box Adversarial Paraphrasing in Text Autoencoder Latent Space
Source: arXiv:2510.24446 source file (2025-10-28)
Supplement: Supplementary file 9 [file system_prompt_simple.tex]

\begin{table}[t!]  
\centering
\captionsetup{type=table} % Force caption type
\tiny 

\begin{lstlisting}[language=,numbers=none,breaklines=true,breakatwhitespace=true,breakindent=0pt,postbreak=\mbox{}]
You need to make a paraphrase of the original query.
It should not be much longer than original one. Also, it should be natural.
Here is the original query:
{orig}
Please provide a paraphrased query that meets the above conditions.
Return only modified query and don't add anything before and after it.
\end{lstlisting}
\caption{\textbf{System Prompt} employed in Qwen3 simple prompt attack.}
\label{table:prompt_simple}

\end{table}
