# Supplementary material for: SPARTA: Evaluating Reasoning Segmentation Robustness through Black-Box Adversarial Paraphrasing in Text Autoencoder Latent Space
Source: arXiv:2510.24446 source file (2025-10-28)
Supplement: Supplementary file 10 [file system_prompt_simple_eval.tex]

\begin{table}[t!]  
\centering
\captionsetup{type=table} % Force caption type
\tiny 

\begin{lstlisting}[language=,numbers=none,breaklines=true,breakatwhitespace=true,breakindent=0pt,postbreak=\mbox{}]
Are the following sentences grammatically correct paraphrases?
Sentence 1: {orig}
Sentence 2: {adv}
Answer only with 1 (means yes) or 0 (means no).
Output ONLY a single integer. No words, no spaces, no punctuation.
\end{lstlisting}
\caption{\textbf{Prompt 1} tested in evaluation of paraphrase detection methods.}
\label{table:prompt_llm_improved_eval}

\end{table}
